# Supplementary material for: MVImgNet: A Large-scale Dataset of Multi-view Images
Source: arXiv:2303.06042 source file (2023-03-10)
Supplement: Supplementary file 1 [file fig_mvs_suppl.tex]

\begin{figure*}[t]
    \centering
   \includegraphics[width=0.5\linewidth]{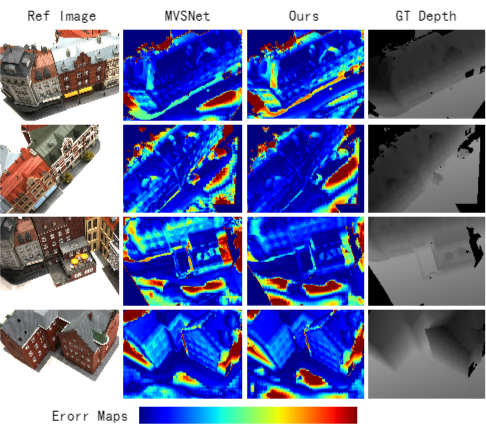}
   \caption{Qualitative results of MVSNet. We visualize the error map of predicted depth and Ground Truth (GT) depth, where \textbf{blue represents the low error}, and \textbf{red indicates the high error}. \textbf{Pretraining MVSNet \cite{yao2018mvsnet} on MVImgNet} improves the performance.}
   \label{fig:sup_mvs}
\end{figure*}
