# Supplementary material for: MVImgNet: A Large-scale Dataset of Multi-view Images
Source: arXiv:2303.06042 source file (2023-03-10)
Supplement: Supplementary file 2 [file fig_nerf_suppl.tex]

\newcommand{\supplgtfigwidth}{0.1\textwidth}
\newcommand{\supplresultswidth}{0.125\textwidth}

\newcommand{\supplinsertimg}[1]{
  \makecell{
  \includegraphics[width=\supplresultswidth]{#1} \\
  }
}

\begin{figure*}[t]
	\centering
	\scriptsize
	\begin{tabular}{@{}c@{\,\,}c@{}c@{}c@{}@{}c@{\,\,}c@{}c@{}c@{}}
		\makecell[c]{
			\includegraphics[trim={0px 0px 0px 0px}, clip, width=\supplgtfigwidth]{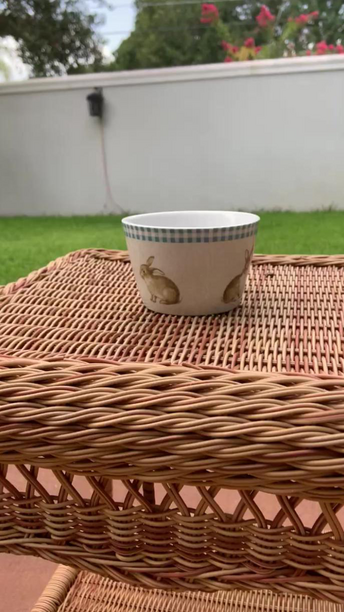}
			\\
			\textit{Bowl}
		}
		&
		\supplinsertimg{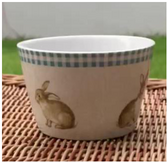} &
		\supplinsertimg{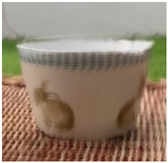} &
		\supplinsertimg{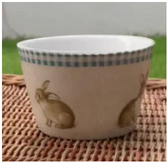} &
		\makecell[c]{
			\includegraphics[trim={0px 0px 0px 0px}, clip, width=\supplgtfigwidth]{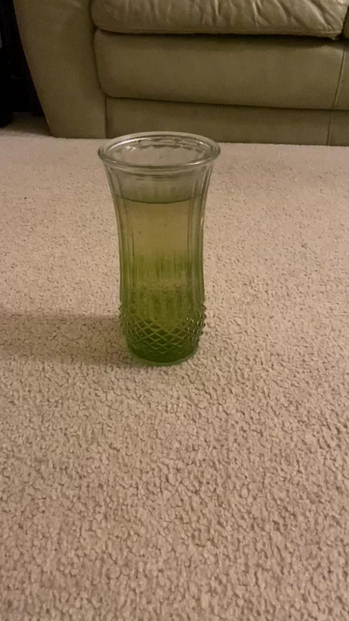}
			\\
			\textit{Vase}
		}
		&
		\supplinsertimg{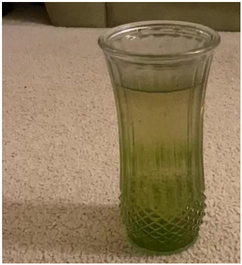} &
		\supplinsertimg{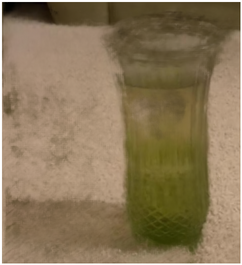} &
		\supplinsertimg{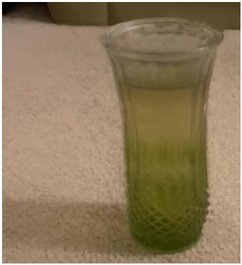} \\
		\makecell[c]{
			\includegraphics[trim={0px 0px 0px 0px}, clip, width=\supplgtfigwidth]{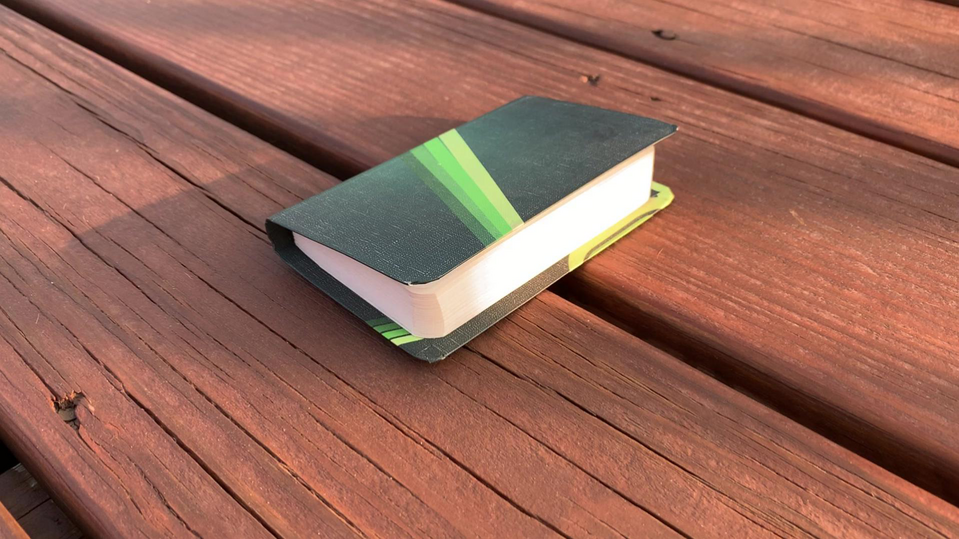}
			\\
			\textit{Book}
		}
		& 
		\supplinsertimg{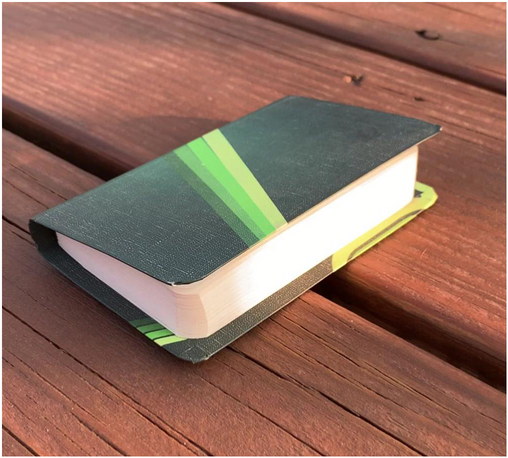} &
		\supplinsertimg{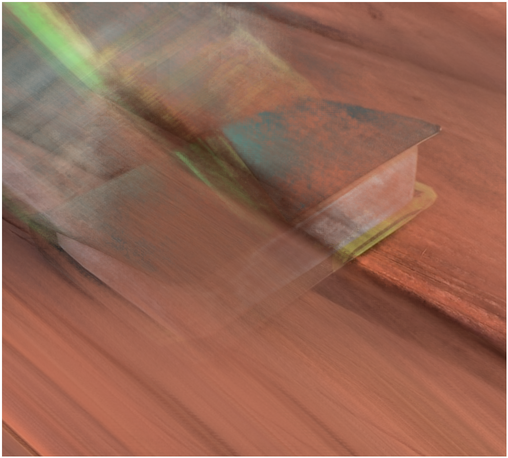} &
		\supplinsertimg{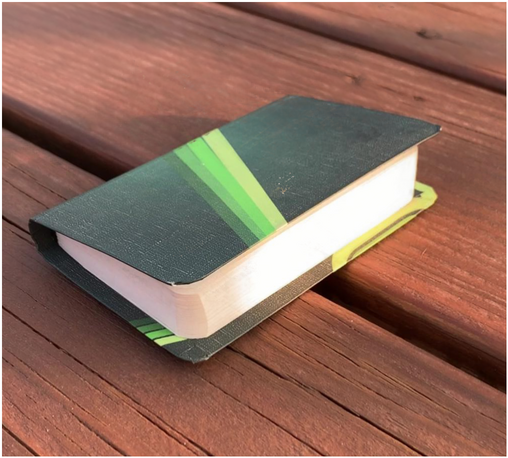} &
		\makecell[c]{
			\includegraphics[trim={0px 0px 0px 0px}, clip, width=\supplgtfigwidth]{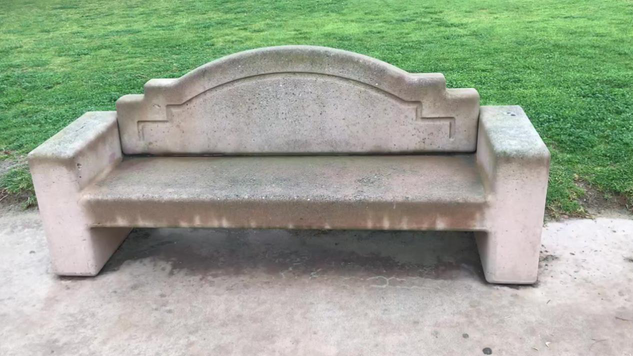}
			\\
			\textit{Bench}
		}
		& 
		\supplinsertimg{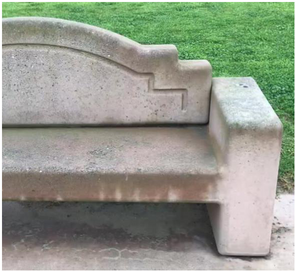} &
		\supplinsertimg{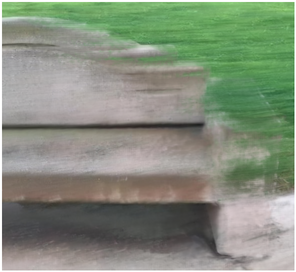} &
		\supplinsertimg{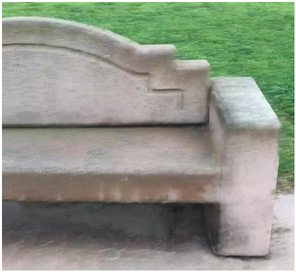} \\
		\makecell[c]{
			\includegraphics[trim={0px 0px 0px 0px}, clip, width=\supplgtfigwidth]{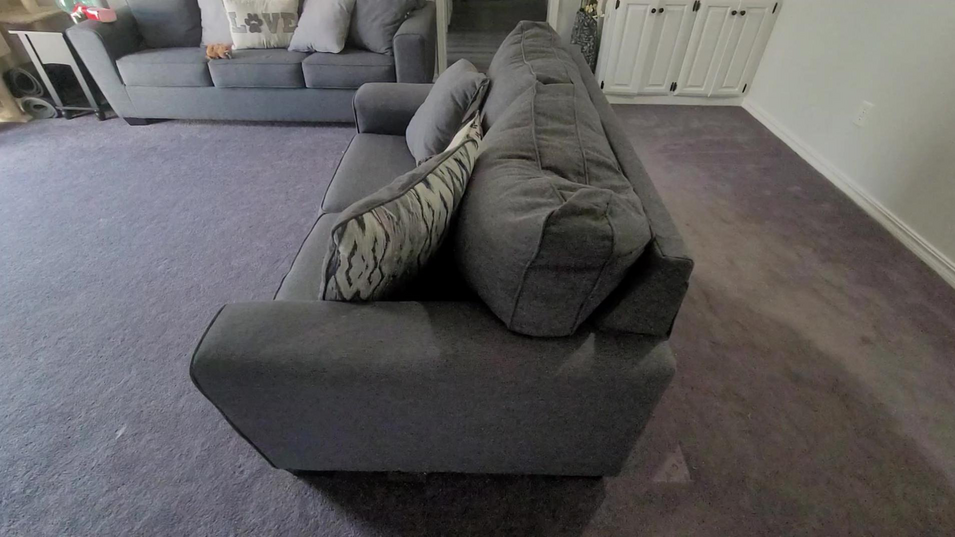}
			\\
			\textit{Couch}
		}
		& 
		\supplinsertimg{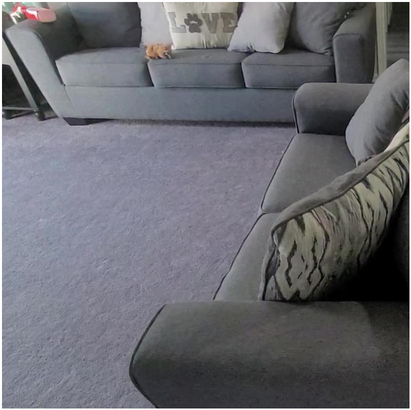} &
		\supplinsertimg{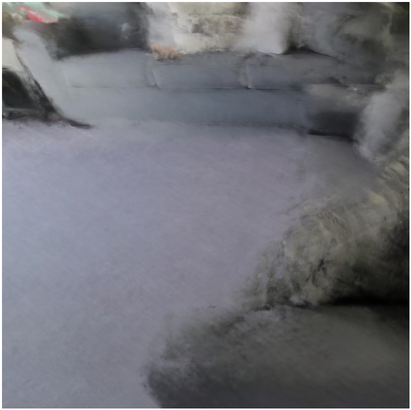} &
		\supplinsertimg{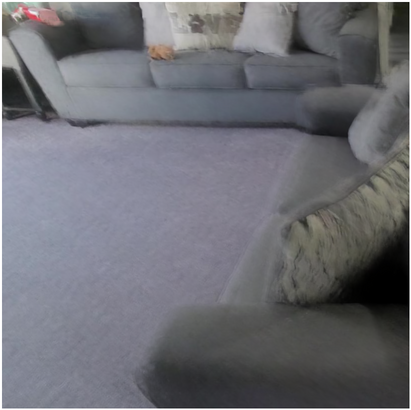} &
		\makecell[c]{
			\includegraphics[trim={0px 0px 0px 0px}, clip, width=\supplgtfigwidth]{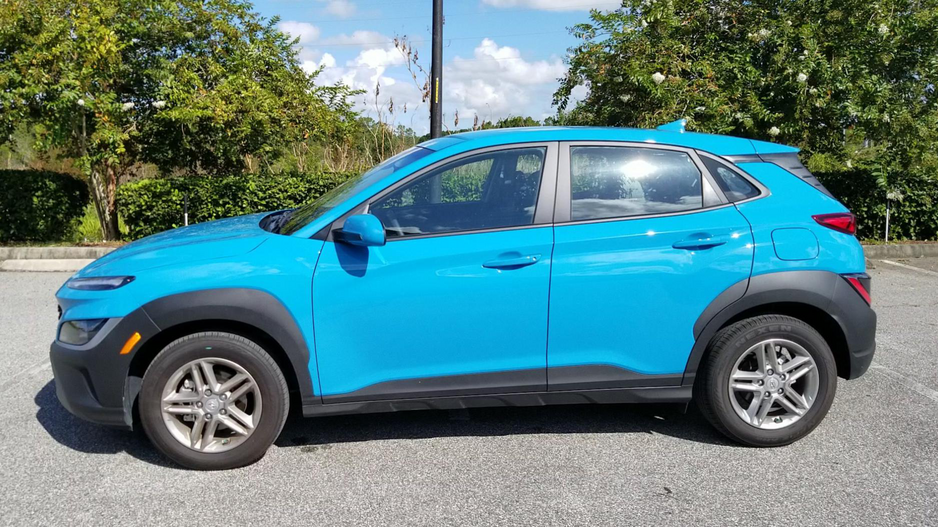}
			\\
			\textit{Car}
		}
		&
		\supplinsertimg{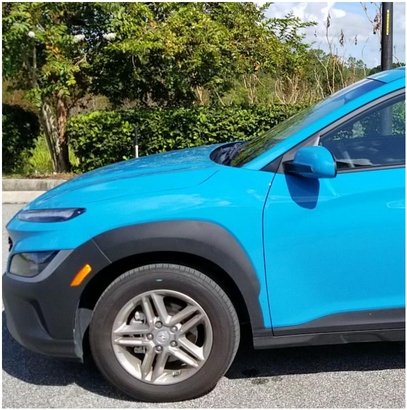} &
		\supplinsertimg{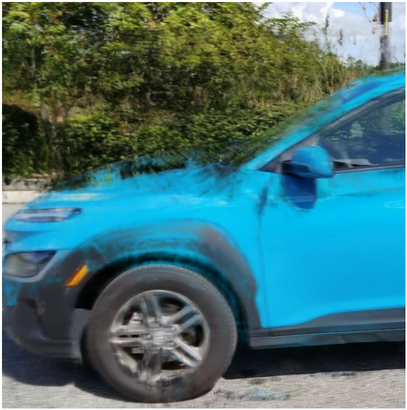} &
		\supplinsertimg{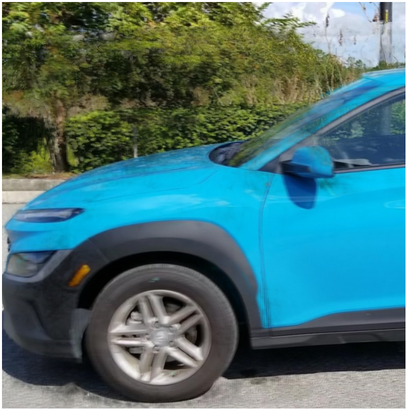} \\
		\makecell[c]{
			\includegraphics[trim={0px 0px 0px 0px}, clip, width=\supplgtfigwidth]{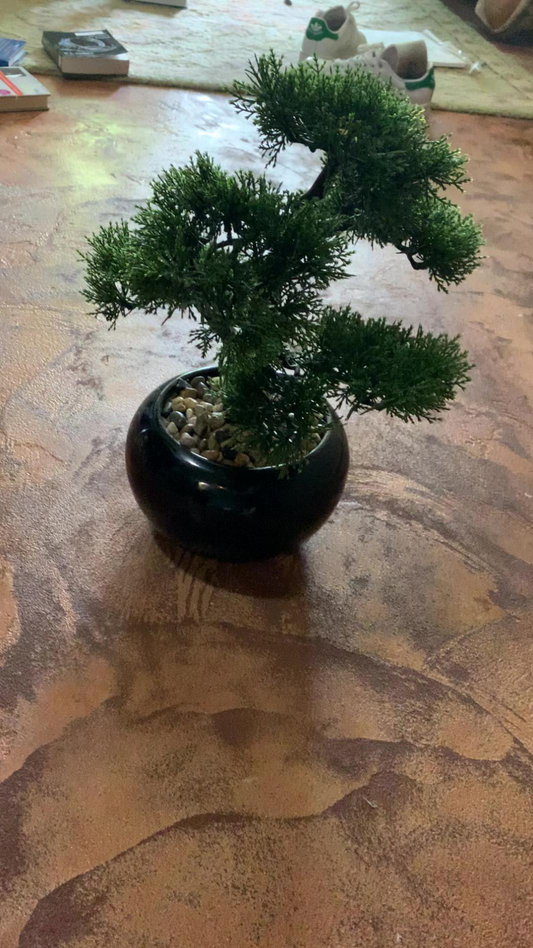}
			\\
			\textit{Plant}
		}
		& 
		\supplinsertimg{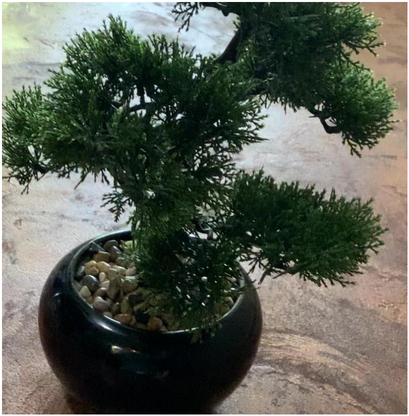} &
		\supplinsertimg{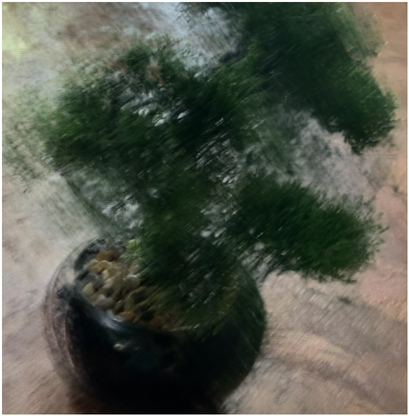} &
		\supplinsertimg{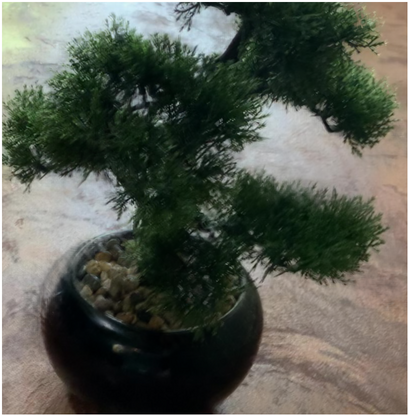} &
		\makecell[c]{
			\includegraphics[trim={0px 0px 0px 0px}, clip, width=\supplgtfigwidth]{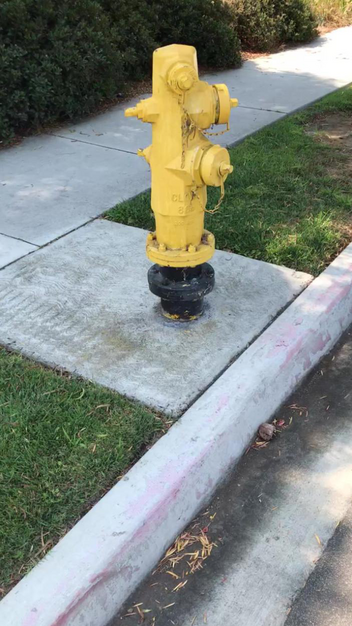}
			\\
			\textit{Hydrant}
		}
		&
		\supplinsertimg{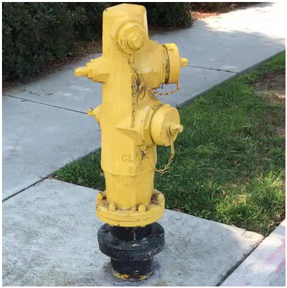} &
		\supplinsertimg{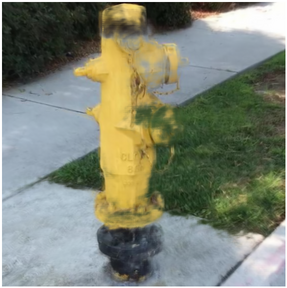} &
		\supplinsertimg{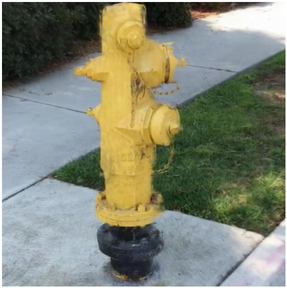} \\
		\makecell[c]{
			\includegraphics[trim={0px 0px 0px 0px}, clip, width=\supplgtfigwidth]{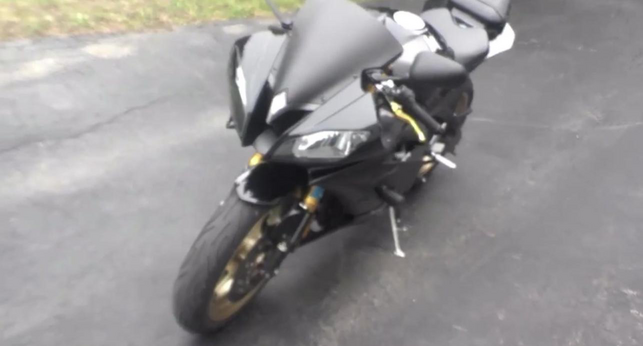}
			\\
			\textit{Motorcycle}
		}
		& 
		\supplinsertimg{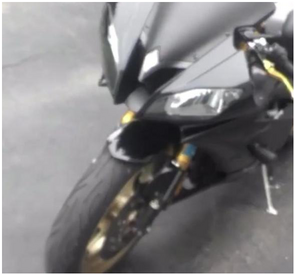} &
		\supplinsertimg{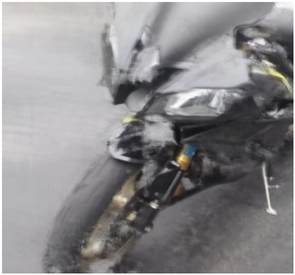} &
		\supplinsertimg{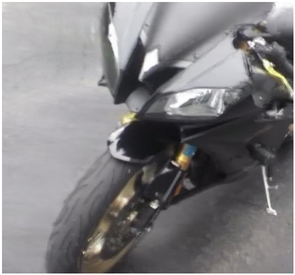} &
		\makecell[c]{
			\includegraphics[trim={0px 0px 0px 0px}, clip, width=\supplgtfigwidth]{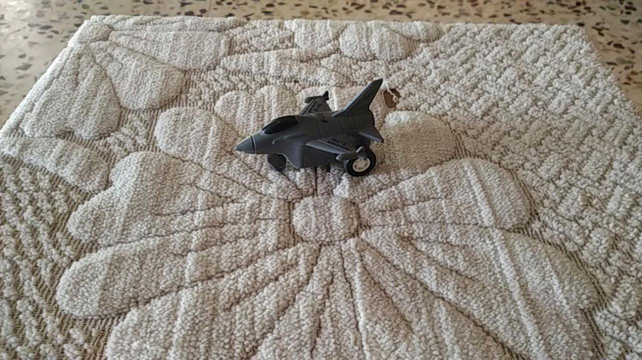}
			\\
			\textit{Toyplane}
		}
		& 
		\supplinsertimg{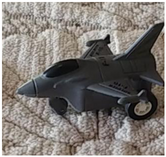} &
		\supplinsertimg{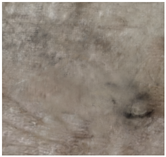} &
		\supplinsertimg{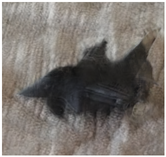} \\
		\makecell[c]{
			\includegraphics[trim={0px 0px 0px 0px}, clip, width=\supplgtfigwidth]{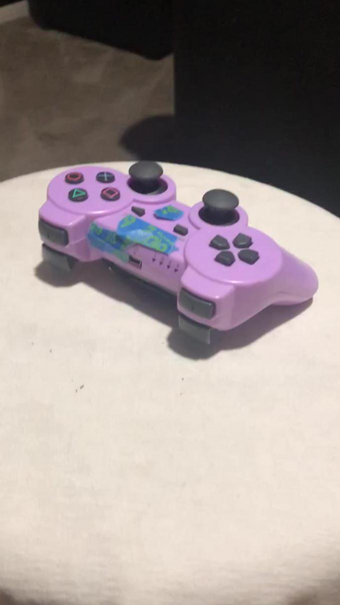}
			\\
			\textit{Remote}
		}
		& 
		\supplinsertimg{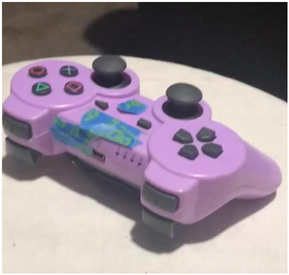} &
		\supplinsertimg{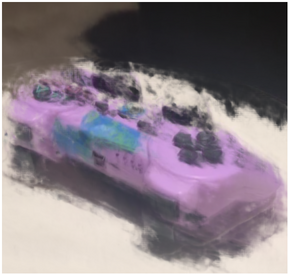} &
		\supplinsertimg{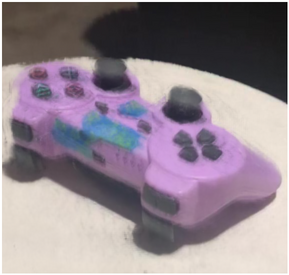} &
		\makecell[c]{
			\includegraphics[trim={0px 0px 0px 0px}, clip, width=\supplgtfigwidth]{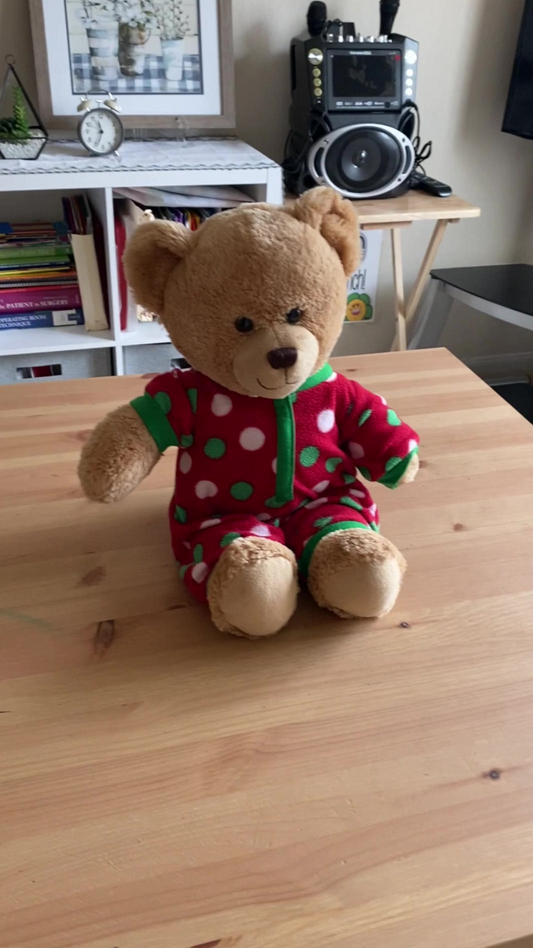}
			\\
			\textit{Teddybear}
		}
		&
		\supplinsertimg{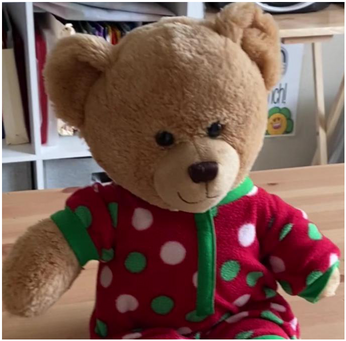} &
		\supplinsertimg{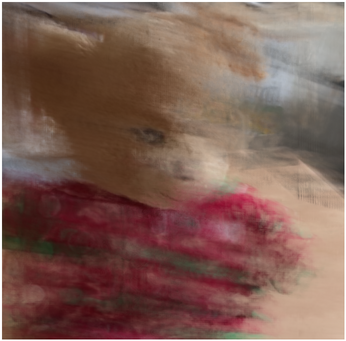} &
		\supplinsertimg{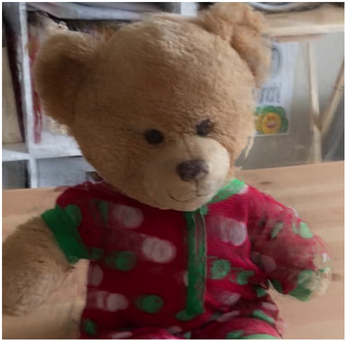} \\
		\makecell[c]{
			\includegraphics[trim={0px 0px 0px 0px}, clip, width=\supplgtfigwidth]{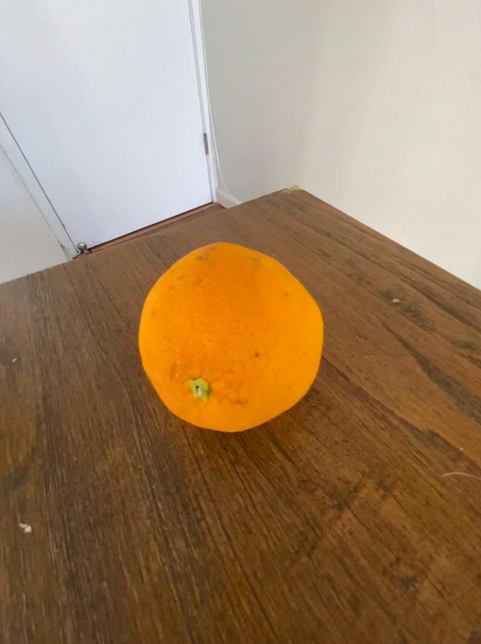}
			\\
			\textit{Orange}
		}
		&
		\supplinsertimg{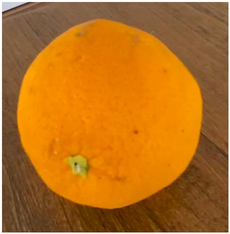} &
		\supplinsertimg{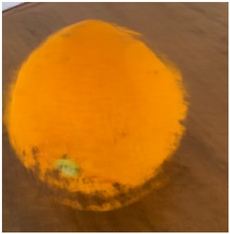} &
		\supplinsertimg{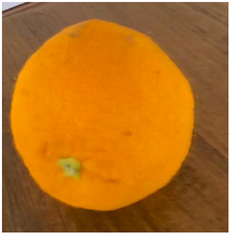} &
		\makecell[c]{
			\includegraphics[trim={0px 0px 0px 0px}, clip, width=\supplgtfigwidth]{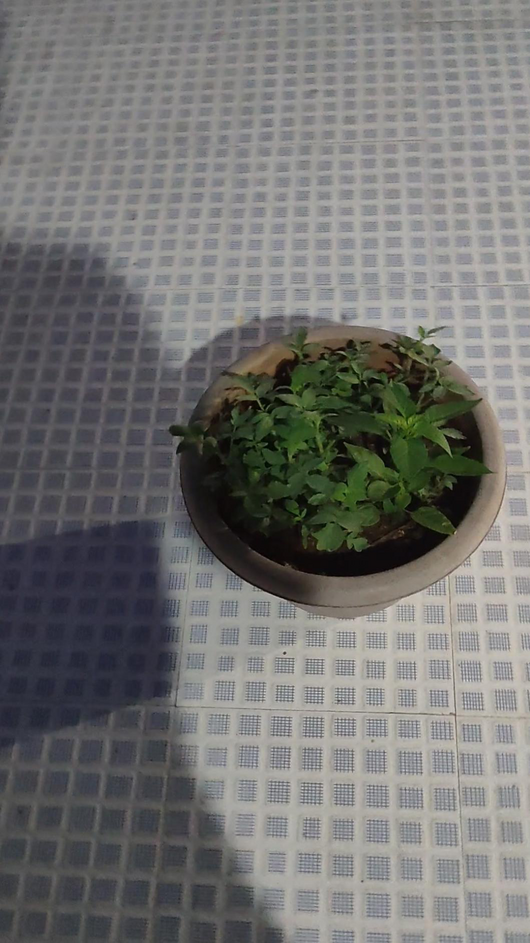}
			\\
			\textit{Plant}
		}
		&
		\supplinsertimg{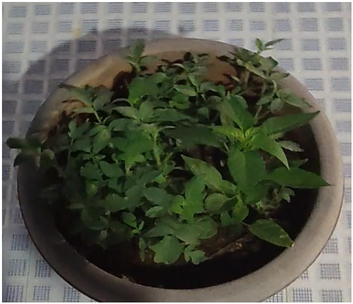} &
		\supplinsertimg{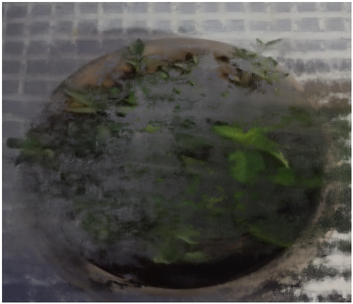} &
		\supplinsertimg{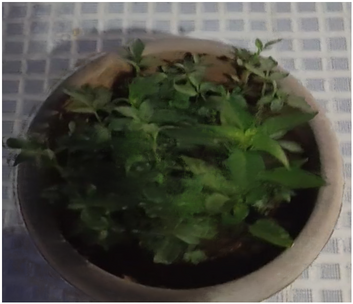} \\
%		\makecell[c]{
%			\includegraphics[trim={0px 0px 0px 0px}, clip, width=\supplgtfigwidth]{imgs/nerf_comp/toyplane_581_86168_170640/gt}
%			\\
%			\textit{Toyplane}
%		}
%		& 
%		\supplinsertimg{imgs/nerf_comp/toyplane_581_86168_170640/crop_gt} &
%		\supplinsertimg{imgs/nerf_comp/toyplane_581_86168_170640/crop_IBRNet} &
%		\supplinsertimg{imgs/nerf_comp/toyplane_581_86168_170640/crop_ours} &
%		\makecell[c]{
%			\includegraphics[trim={0px 0px 0px 0px}, clip, width=\supplgtfigwidth]{imgs/nerf_comp/plant_374_42005_84358/gt}
%			\\
%			\textit{Plant}
%		}
%		&
%		\supplinsertimg{imgs/nerf_comp/plant_374_42005_84358/crop_gt} &
%		\supplinsertimg{imgs/nerf_comp/plant_374_42005_84358/crop_IBRNet} &
%		\supplinsertimg{imgs/nerf_comp/plant_374_42005_84358/crop_ours} \\
%		\makecell[c]{
%			\includegraphics[trim={0px 0px 0px 0px}, clip, width=\supplgtfigwidth]{imgs/nerf_comp/toyplane_581_86168_170640/gt}
%			\\
%			\textit{Book}
%		}
%		& 
%		\supplinsertimg{imgs/nerf_comp/toyplane_581_86168_170640/crop_gt} &
%		\supplinsertimg{imgs/nerf_comp/toyplane_581_86168_170640/crop_IBRNet} &
%		\supplinsertimg{imgs/nerf_comp/toyplane_581_86168_170640/crop_ours} &
%		\makecell[c]{
%			\includegraphics[trim={0px 0px 0px 0px}, clip, width=\supplgtfigwidth]{imgs/nerf_comp/umbrella_586_87527_173920/gt}
%			\\
%			\textit{Cake}
%		}
%		&
%		\supplinsertimg{imgs/nerf_comp/umbrella_586_87527_173920/crop_gt} &
%		\supplinsertimg{imgs/nerf_comp/umbrella_586_87527_173920/crop_IBRNet} &
%		\supplinsertimg{imgs/nerf_comp/umbrella_586_87527_173920/crop_ours} \\
		& Ground Truth  &  Scratch & \textbf{MVImgNet-pretrained} & & Ground Truth & Scratch & \textbf{MVImgNet-pretrained}
	\end{tabular}
%	\vspace{-0.2cm}
	\caption{More qualitative comparison on real-world 360$^\circ$ objects~\cite{co3d} of \textbf{MVImgNet-pretrained} IBRNet~\cite{wang2021ibrnet} model and the \textbf{train-from-scratch} model.}
	
	% \vspace{-0.5em}
	\label{fig:nerf_suppl}
\end{figure*}
